# Supplementary material for: Deep learning of multi-resolution X-Ray micro-CT images for multi-scale modelling
Source: arXiv:2111.01270 ancillary file (2022-03-16)
Supplement: Supplementary file 1 [file supporting_information.pdf]

# Supporting information for 'Deep learning of multi-resolution X-Ray micro-CT images for multi-scale modelling'

Samuel J. Jackson,[1,*] Yufu Niu,[2] Sojwal Manoorkar,[3] Peyman Mostaghimi,[2] and Ryan T. Armstrong[2]

[1]*CSIRO Energy, Private Bag 10, Clayton South, Victoria 3169, Australia*
[2]*School of Minerals and Energy Resources Engineering, University of New South Wales, Sydney, New South Wales 2052, Australia*
[3]*Department of Earth Science & Engineering, Imperial College London, London, SW72BP, UK*

(Dated: October 26, 2021)

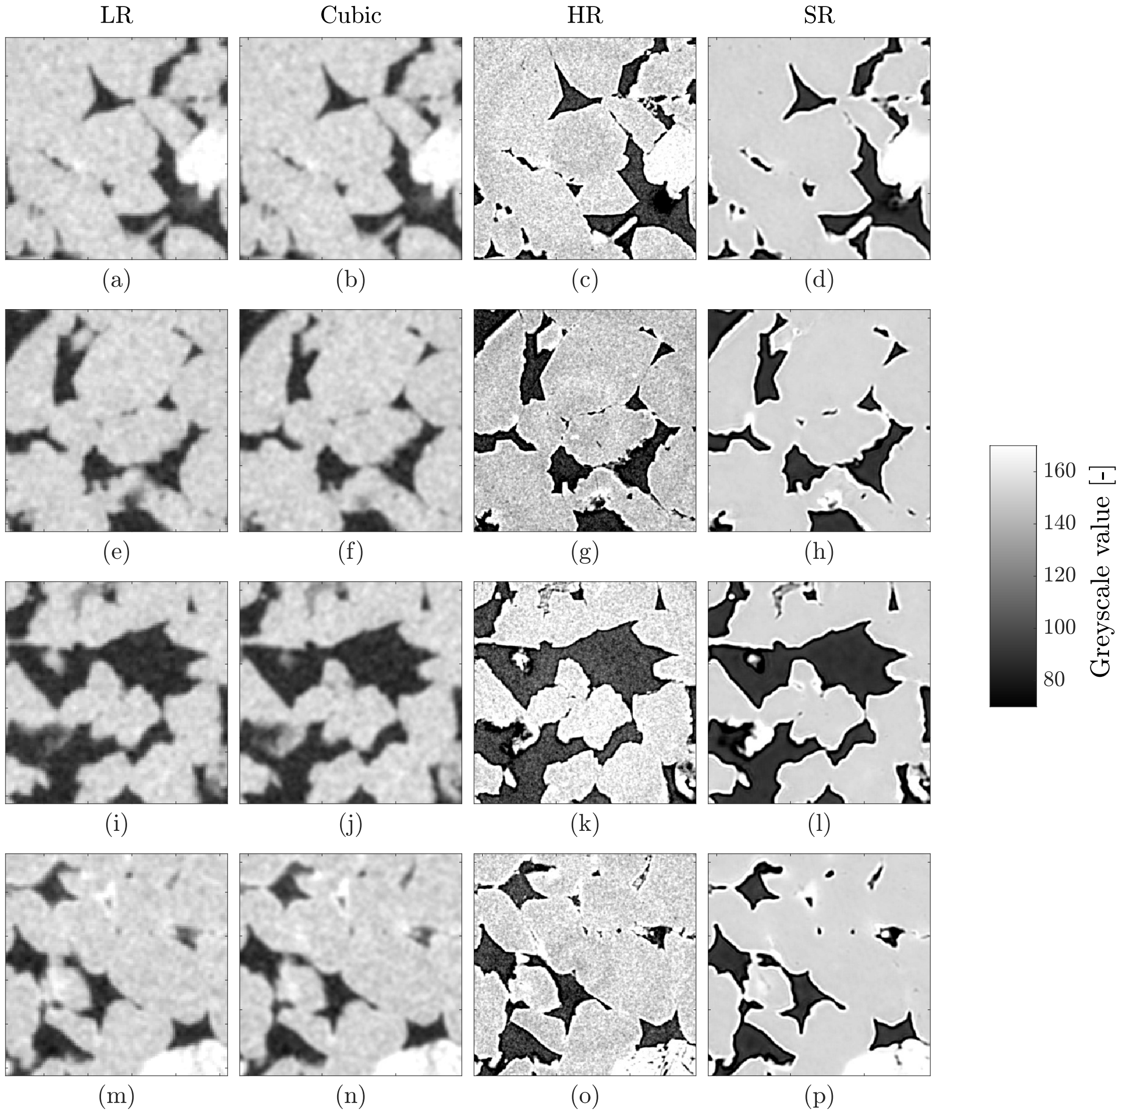


FIG. S1. Comparisons of LR, Cubic, HR and SR raw, nomalised images. Region shown is a 600 x 600 $\mu$m 2D crop from the first slice, centred on pixel 113/225. (a-d) core 1 subvolume 1. (e-h) core 1 subvolume 2. (i-l) core 2 subvolume 1. (m-p) core 2 subvolume 2. The columns from left to right are LR, Cubic, HR and SR images, respectively.

* Corresponding author email: samuel.jackson@csiro.au

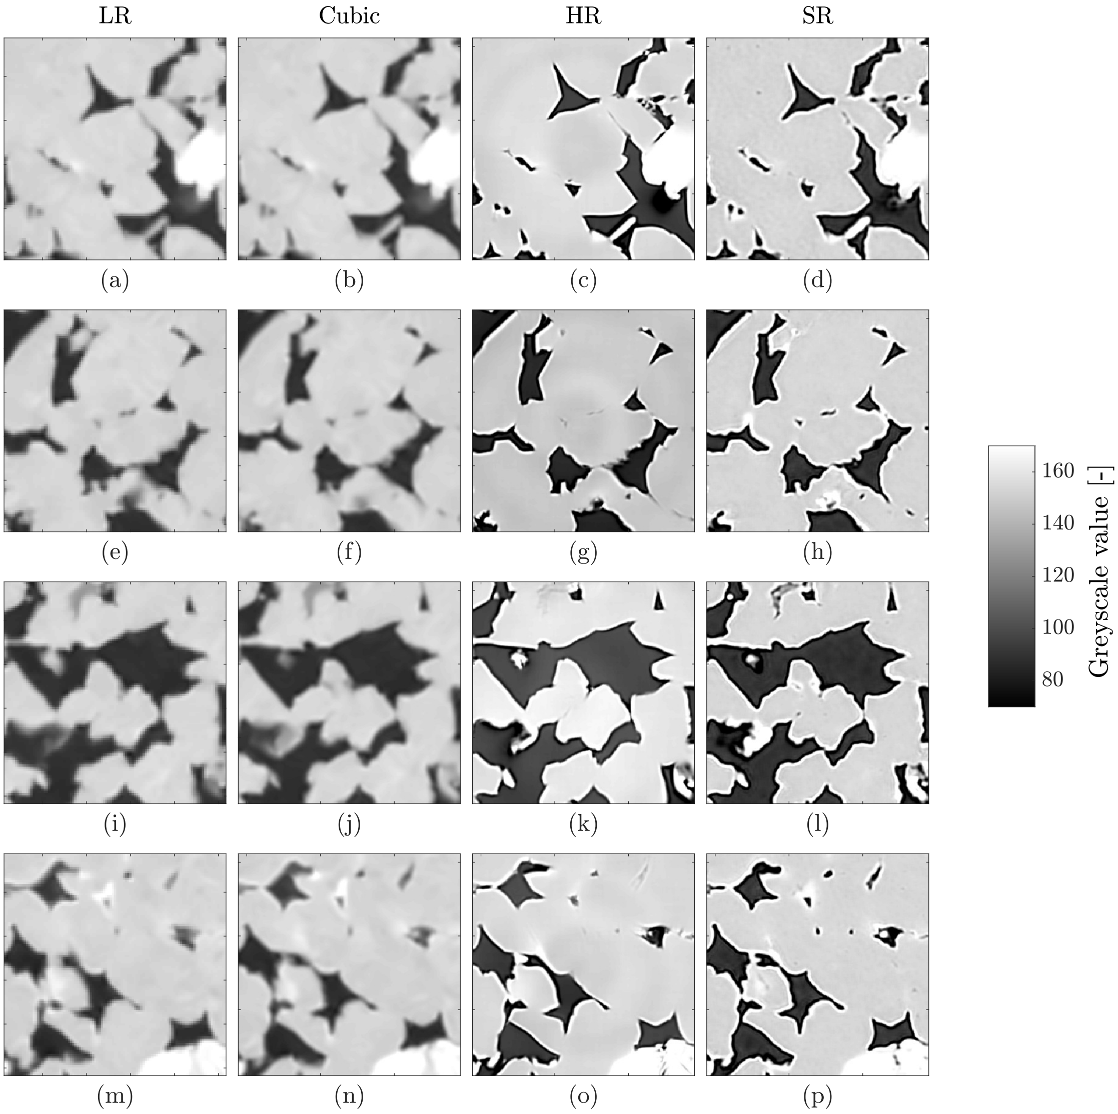


FIG. S2. Comparisons of LR, Cubic, HR and SR filtered images. Region shown is a 600 x 600 $\mu$m 2D crop from the first slice, centred on pixel 113/225. (a-d) core 1 subvolume 1. (e-h) core 1 subvolume 2. (i-l) core 2 subvolume 1. (m-p) core 2 subvolume 2. The columns from left to right are LR, Cubic, HR and SR images, respectively.

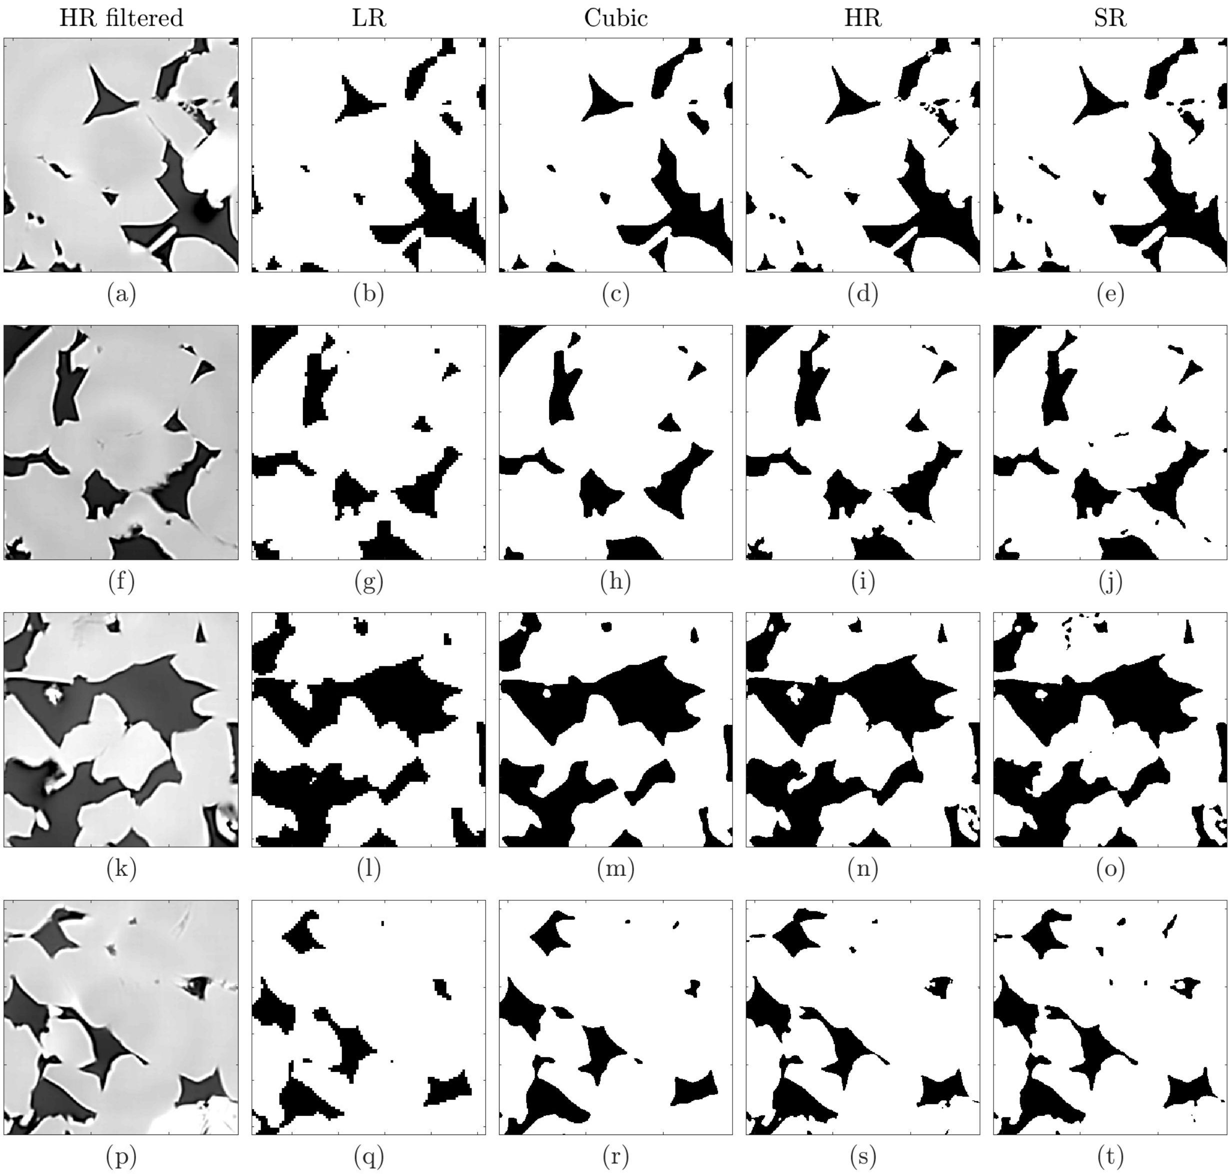


FIG. S3. Comparisons of LR, Cubic, HR and SR segmented images. The HR filtered image is shown for comparison on the far left column. Segmentation threshold is the base 117 greyscale value. Region shown is a 600 x 600 $\mu$m 2D crop from the first slice, centred on pixel 113/225. (a-e) core 1 subvolume 1. (f-j) core 1 subvolume 2. (k-o) core 2 subvolume 1. (p-t) core 2 subvolume 2. The columns from left to right are HR filtered, LR, Cubic, HR and SR images, respectively.

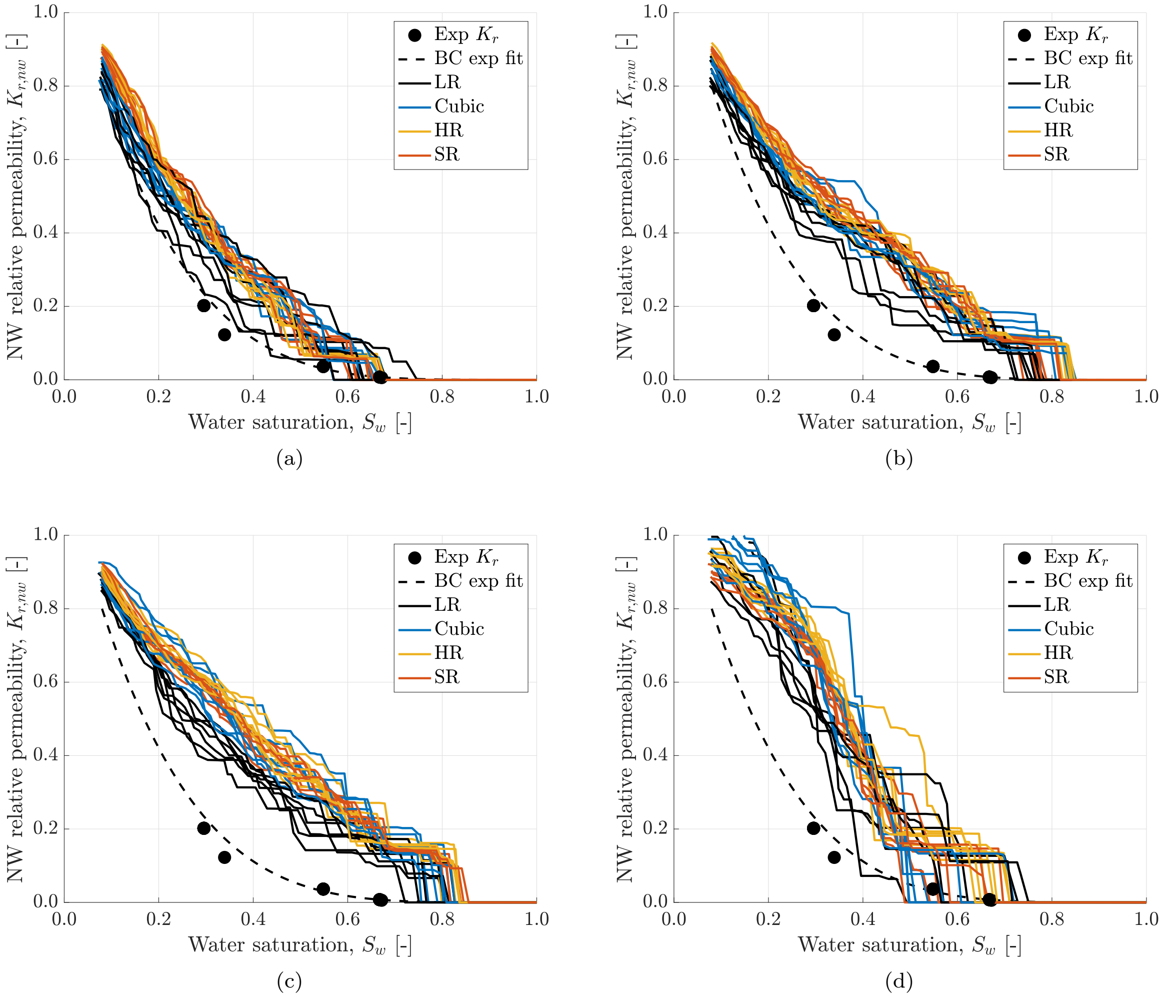


FIG. S4. Pore-network model simulations of the non-wetting relative permeability. (a) core 1 subvolume 1. (b) core 1 subvolume 2. (c) core 2 subvolume 1. (d) core 2 subvolume 2. Each line represent a flow simulation on one of seven different segmentation thresholds from -15% to +15% around the base threshold of 117 greyscale value. The exp Kr data is from the core averaged multiphase flow experiments. There is a Brooks-Corey (BC) function fit to the experimental data also shown from [1].

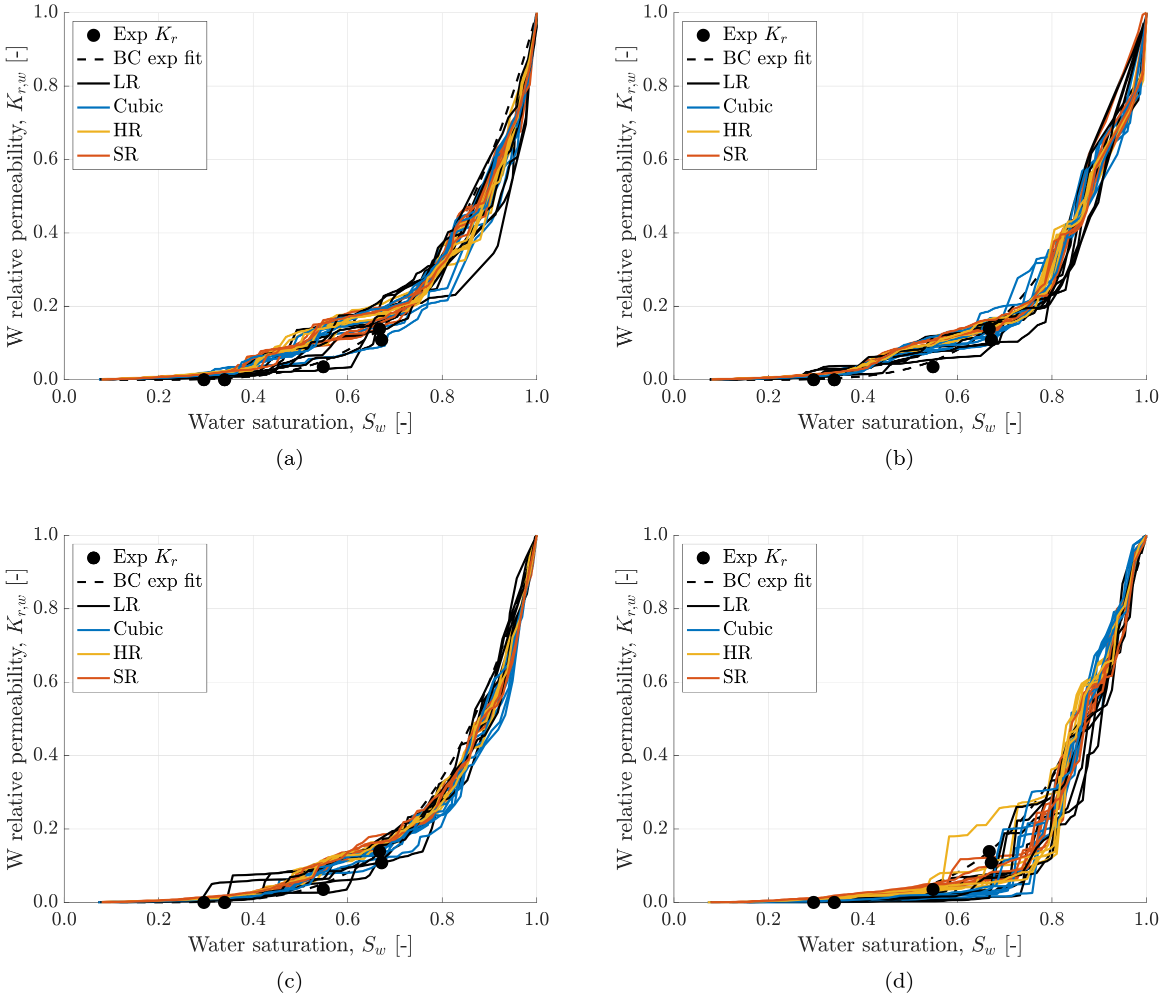


FIG. S5. Pore-network model simulations of the wetting relative permeability. (a) core 1 subvolume 1. (b) core 1 subvolume 2. (c) core 2 subvolume 1. (d) core 2 subvolume 2. Each line represent a flow simulation on one of seven different segmentation thresholds from -15% to +15% around the base threshold of 117 greyscale value. The exp Kr data is from the core averaged multiphase flow experiments. There is a Brooks-Corey (BC) function fit to the experimental data also shown from [1].

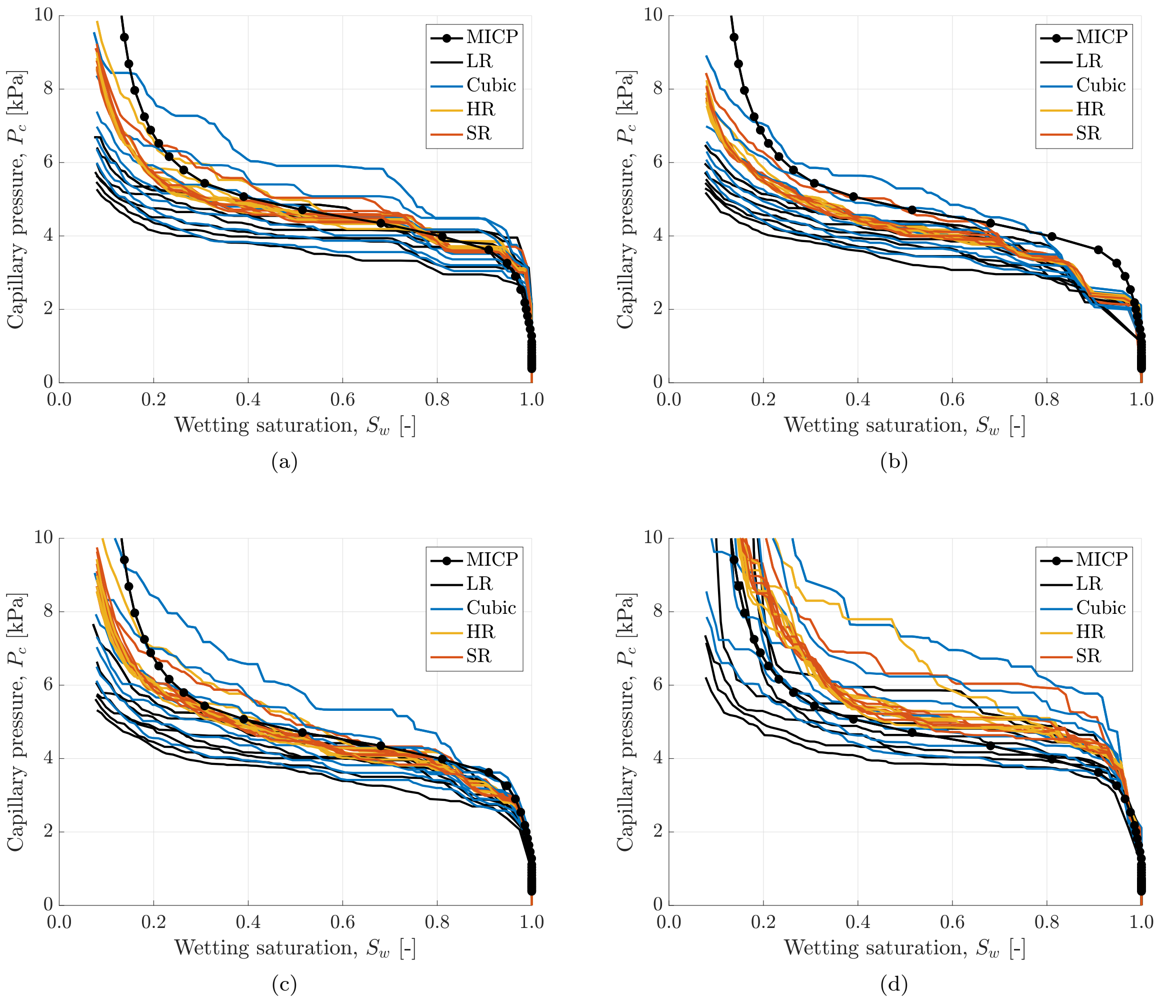


FIG. S6. Pore-network model simulations of the capillary pressure. (a) core 1 subvolume 1. (b) core 1 subvolume 2. (c) core 2 subvolume 1. (d) core 2 subvolume 2. Each line represent a flow simulation on one of seven different segmentation thresholds from -15% to +15% around the base threshold of 117 greyscale value. The MICP data is from a sister core.

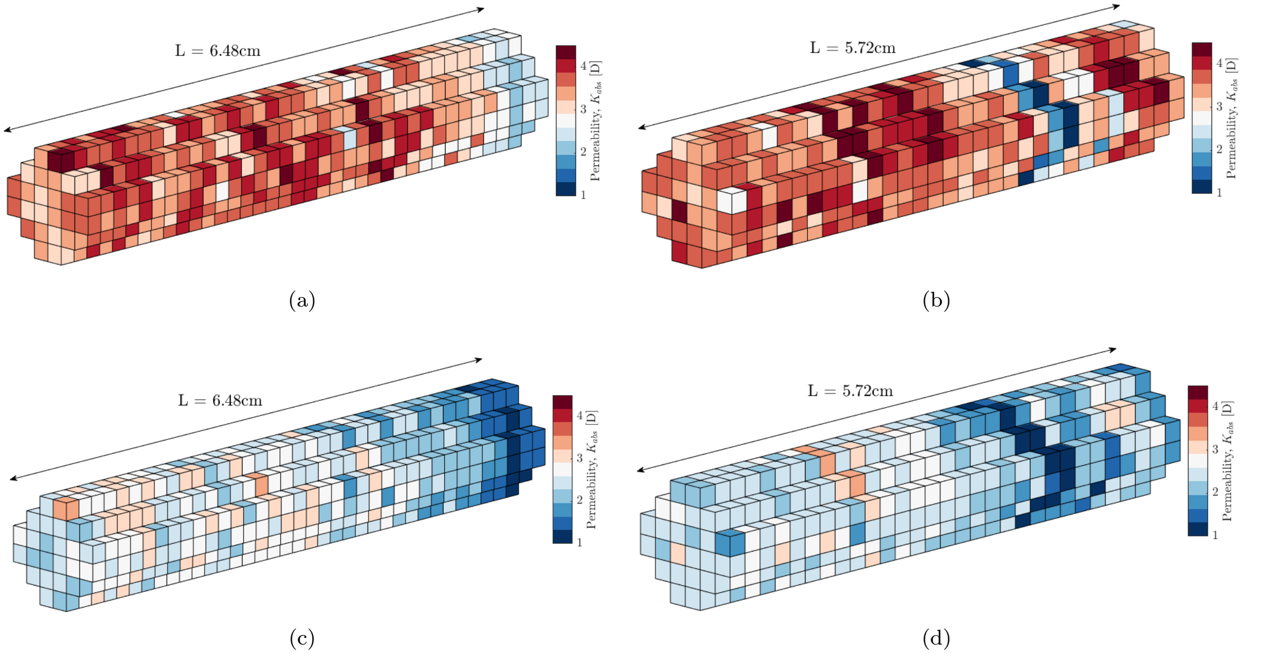


FIG. S7. Voxelised whole core permeability results from the PNM using the LR HT and SR HT images. (a, c) Core 1, LR and SR models, respectively. (b, d) Core 2 LR and SR models, respectively. HT images are found in SI Figure S7.

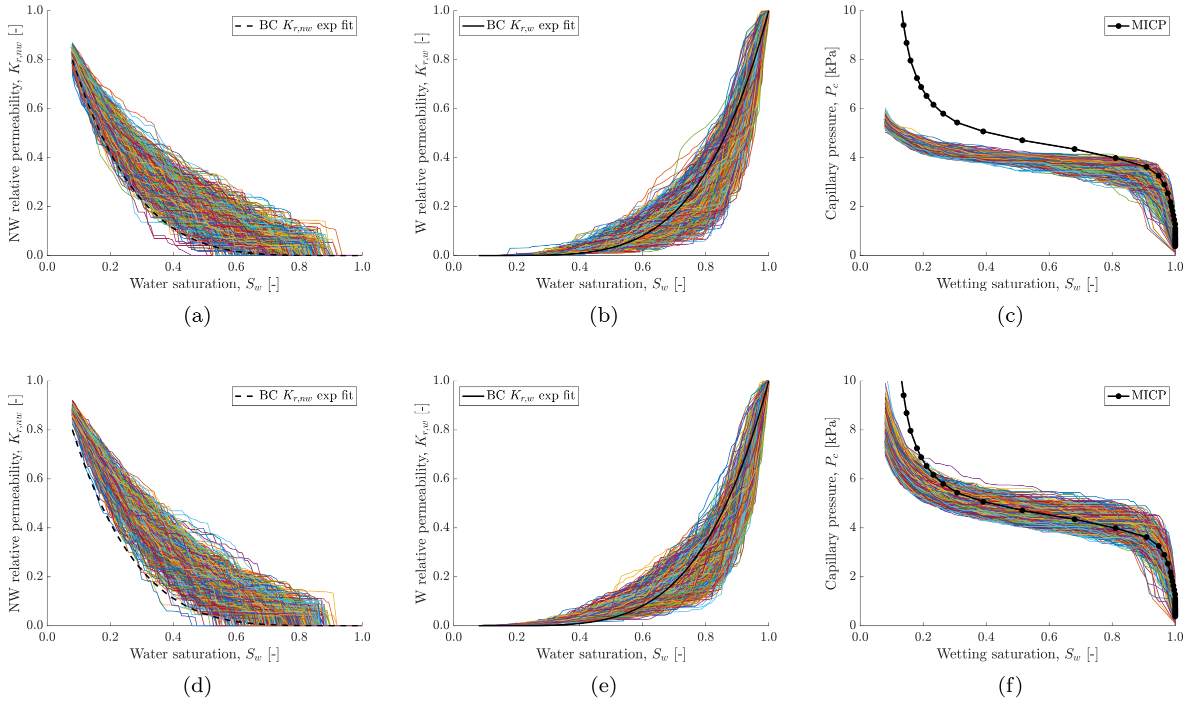


FIG. S8. Pore-network generated relative permeability and capillary pressure for core 1. Each line represents a different subvolume in core 1. The top row show results from the low resolution, high threshold images, bottom row show resuilts from the super resolution, high threshold images. Columns from left to right show non-wetting relative permeability, wetting relative permeability and capillary pressure, respectively. There is a Brooks-Corey (BC) function fit to the experimental relative permeability data also shown from [1]. The MICP data is from a sister core.

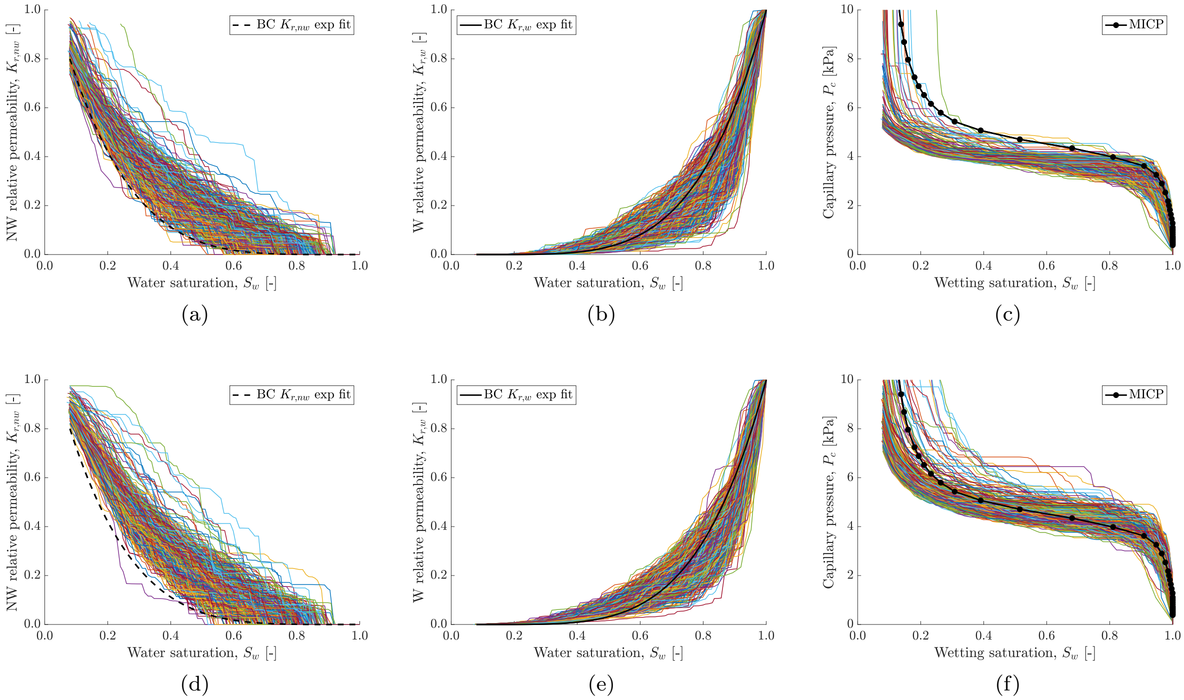


FIG. S9. Pore-network generated relative permeability and capillary pressure for core 2. Each line represents a different subvolume in core 1. The top row show results from the low resolution, high threshold images, bottom row show resuilts from the super resolution, high threshold images. Columns from left to right show non-wetting relative permeability, wetting relative permeability and capillary pressure, respectively. There is a Brooks-Corey (BC) function fit to the experimental relative permeability data also shown from [1]. The MICP data is from a sister core.

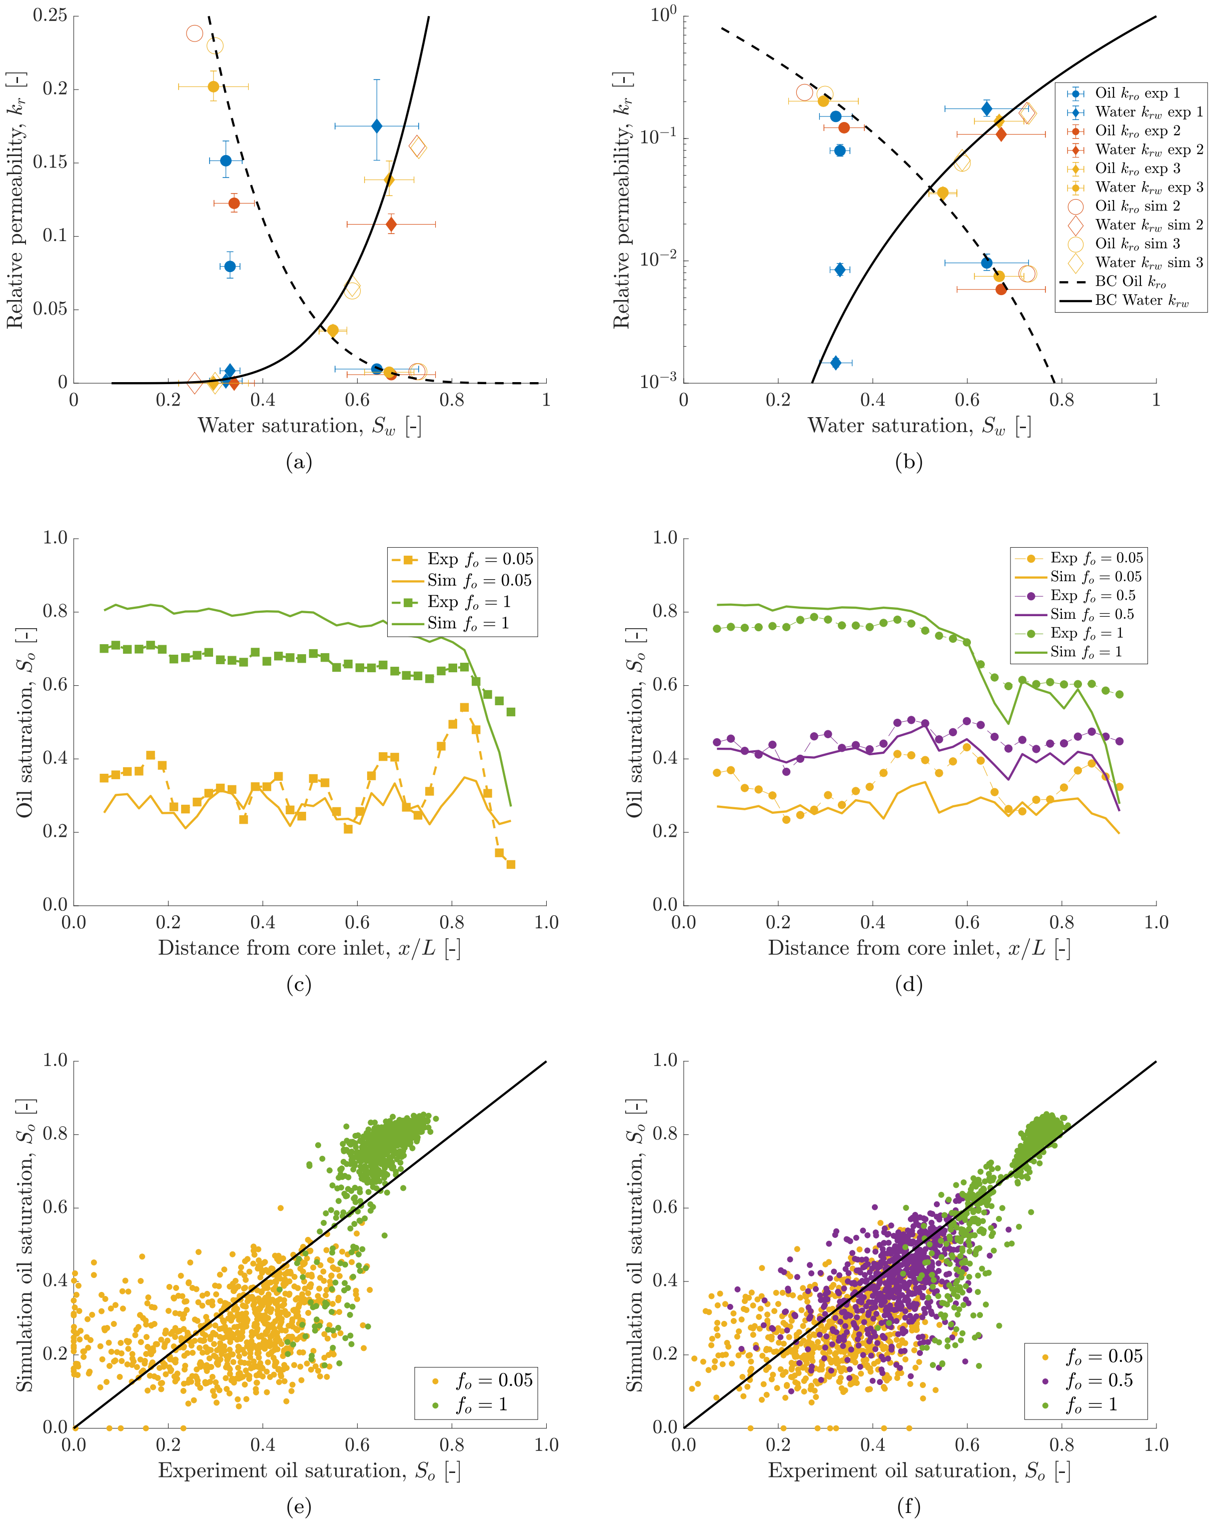


FIG. S10. Whole core simulation results using petrophysical properties derived from the low resolution, low threshold images. (a,b) Linear and logarithmic relative permeability results. Open symbols are the simulations, closed symbols are the experiment. Note, here we simulate exp 2 and exp 3 from [1] (c-f) Whole core saturations for the experiments and simulations. Left column is core 1, right column is core 2. (c, d) Slice average saturations. (e, f) Voxelised saturations.

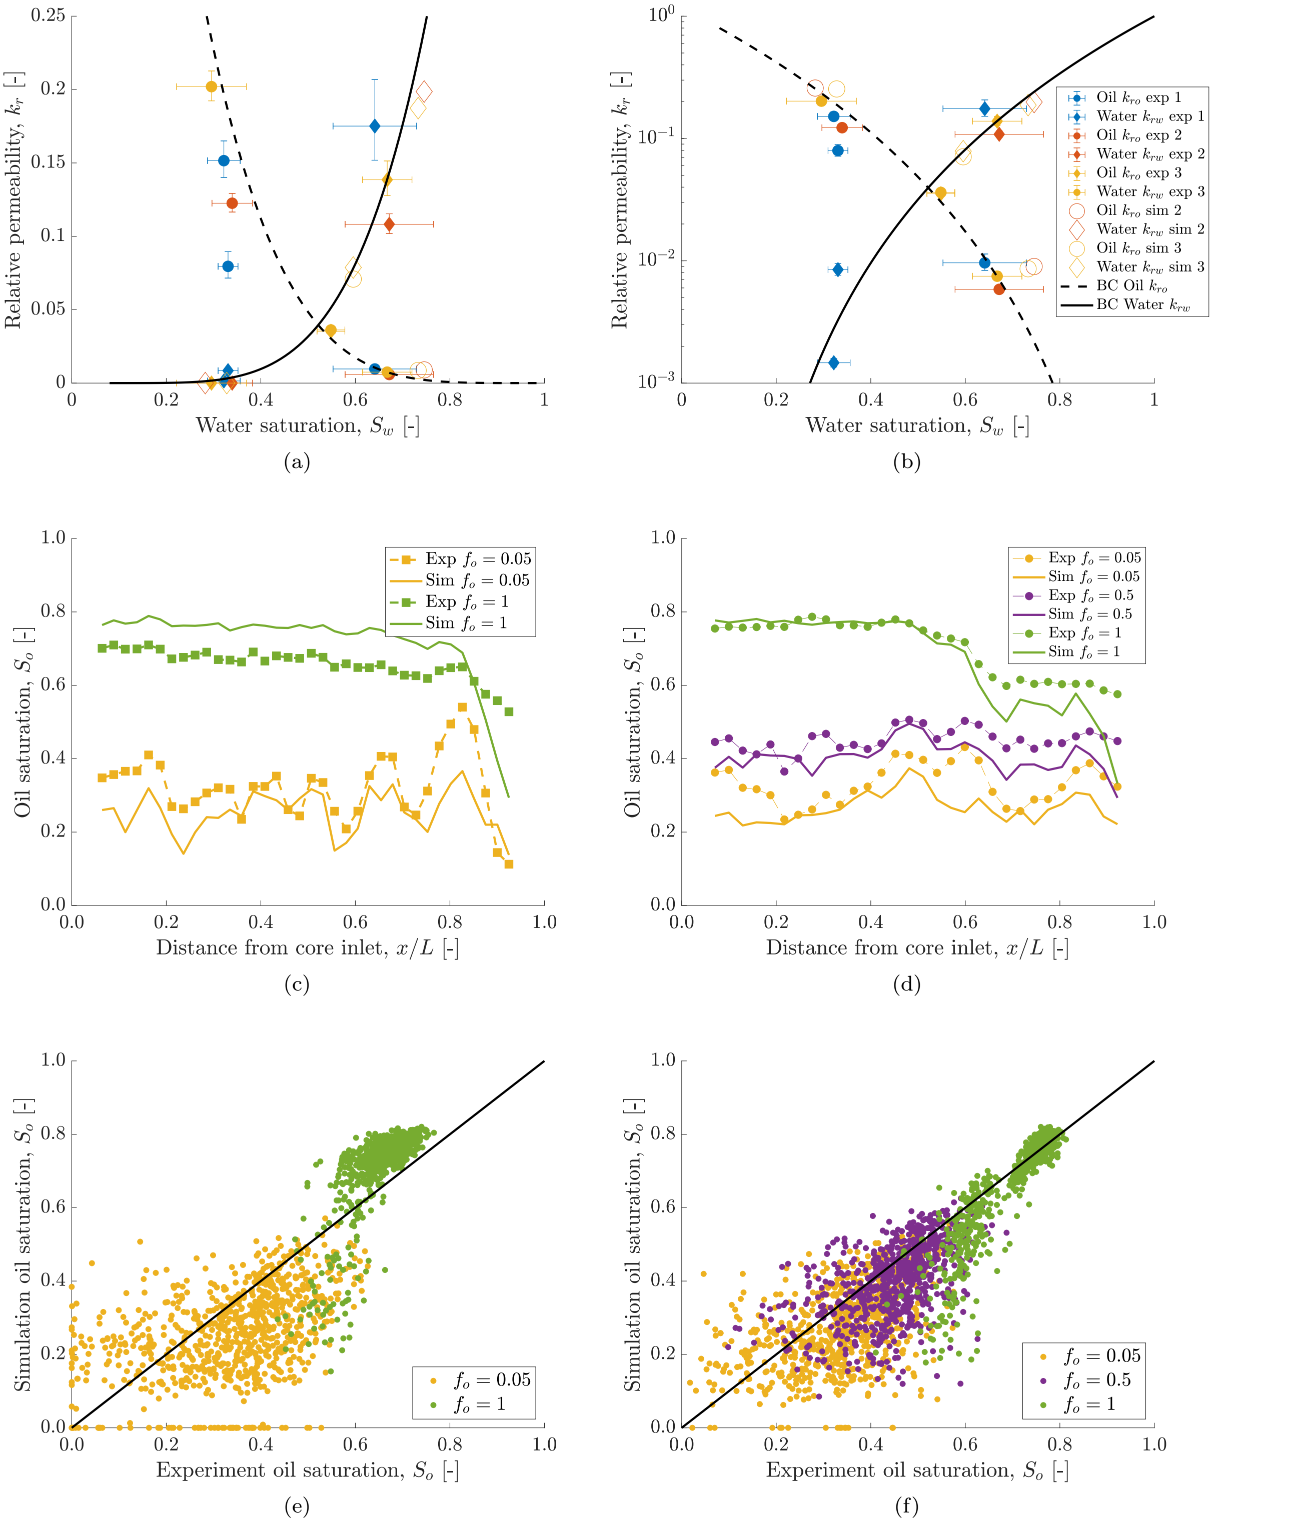


FIG. S11. Whole core simulation results using petrophysical properties derived from the low resolution, high threshold images. (a, b) Linear and logarithmic relative permeability results. Open symbols are the simulations, closed symbols are the experiment. Note, here we simulate exp 2 and exp 3 from [1] (c-f) Whole core saturations for the experiments and simulations. Left column is core 1, right column is core 2. (c, d) Slice average saturations. (e, f) Voxelised saturations.

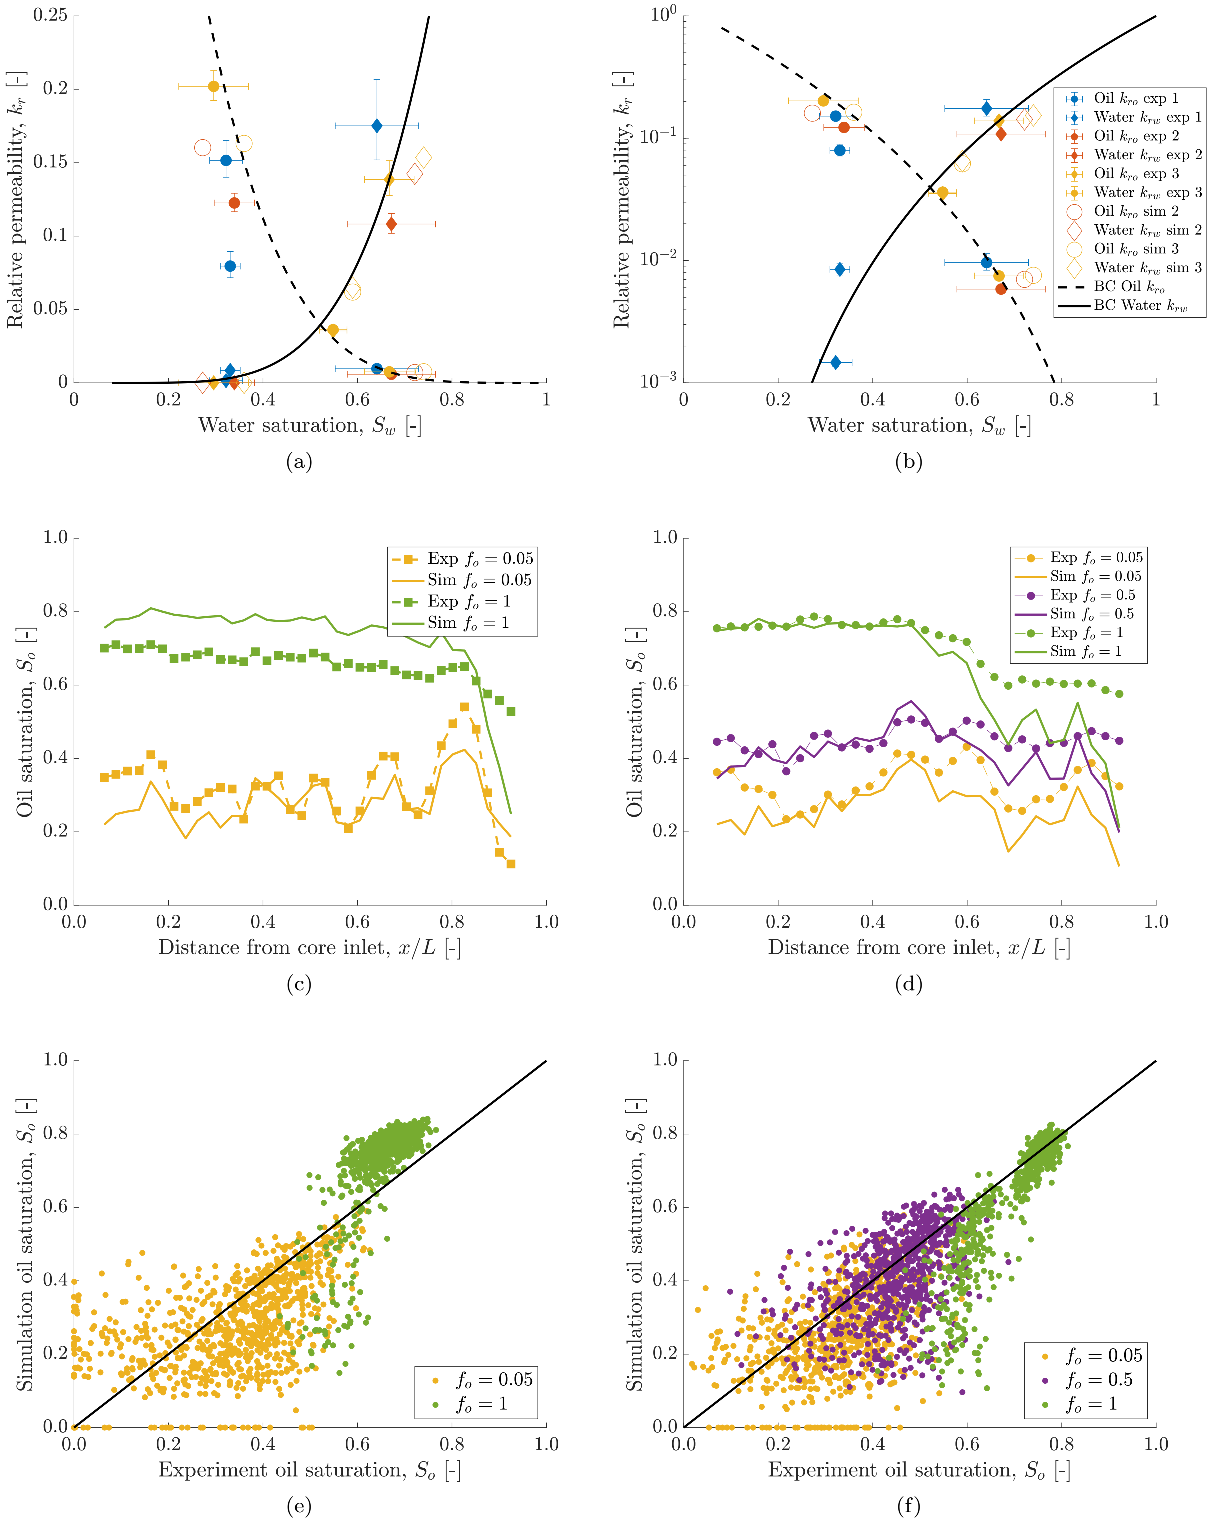


FIG. S12. Whole core simulation results using petrophysical properties derived from the super resolution, high threshold images. (a, b) Linear and logarithmic relative permeability results. Open symbols are the simulations, closed symbols are the experiment. Note, here we simulate exp 2 and exp 3 from [1] (c-f) Whole core saturations for the experiments and simulations. Left column is core 1, right column is core 2. (c, d) Slice average saturations. (e, f) Voxelised saturations.

TABLE S1. Multiphase flow simulation results compared to experiments. Results are shown for models derived from the high threshold images. Lines showing simulation error [%] are in bold.

| | **Core 1** | | | | **Core 2** | | | | | |
|---|---|---|---|---|---|---|---|---|---|---|
| | **LR** | | **SR** | | **LR** | | | **SR** | | |
| **Fractional flow oil, $f_o$ [-]** | 0.05 | 1 | 0.05 | 1 | 0.05 | 0.5 | 1 | 0.05 | 0.5 | 1 |
| $S_w$ av. exp [-] | 0.672 | 0.339 | 0.672 | 0.339 | 0.667 | 0.548 | 0.296 | 0.667 | 0.548 | 0.296 |
| $S_w$ av. sim [-] | 0.746 | 0.282 | 0.721 | 0.272 | 0.733 | 0.596 | 0.328 | 0.740 | 0.590 | 0.360 |
| **$S_w$ av. err [%]** | **11.0** | **-16.8** | **7.4** | **-19.7** | **9.8** | **8.6** | **10.9** | **10.9** | **7.6** | **21.8** |
| $k_{ro}$ exp [-] | 0.00584 | 0.123 | 0.00584 | 0.123 | 0.00748 | 0.0362 | 0.202 | 0.00748 | 0.0362 | 0.202 |
| $k_{ro}$ sim [-] | 0.00898 | 0.259 | 0.00701 | 0.160 | 0.00861 | 0.0709 | 0.254 | 0.00757 | 0.0618 | 0.163 |
| **$k_{ro}$ err [%]** | **53.8** | **111.0** | **20.1** | **30.8** | **15.1** | **95.7** | **25.8** | **1.2** | **70.7** | **-19.3** |
| $k_{rw}$ exp [-] | 0.108 | 0 | 0.108 | 0 | 0.139 | 0.0353 | 0 | 0.139 | 0.0353 | 0 |
| $k_{rw}$ sim [-] | 0.199 | 0 | 0.142 | 0 | 0.187 | 0.0788 | 0 | 0.154 | 0.0649 | 0 |
| **$k_{rw}$ err [%]** | **83.6** | **0** | **31.6** | **0** | **35.2** | **122.9** | **0** | **10.8** | **83.6** | **0** |

## REFERENCES

[1] S. J. Jackson, Q. Lin, and S. Krevor, Representative elementary volumes, hysteresis, and heterogeneity in multiphase flow from the pore to continuum scale, Water Resources Research **56**, 10.1029/2019wr026396 (2020).
